# Supplementary material for: Exploiting HDMI and USB Ports for GPU Side-Channel Insights
Source: arXiv:2410.02539 source file (2024-10-03)
Supplement: Supplementary file 1 [file appendix.tex]

\appendix
